# Supplementary material for: Rydberg excitation of cold atoms inside a hollow core fiber
Source: arXiv:1706.07666 ancillary file (2017-10-04)
Supplement: Supplementary file 1 [file Supplement.pdf]

# Supplemental Material: Rydberg excitation of cold atoms inside a hollow core fiber

Maria Langbecker,[1] Mohammad Noaman,[1] Niels Kjærgaard,[2] Fetah Benabid,[3] and Patrick Windpassinger[1,*]

[1]*Institut für Physik, Johannes Gutenberg-Universität Mainz, 55122 Mainz, Germany*
[2]*Department of Physics, QSO — Centre for Quantum Science, and Dodd-Walls Centre for Photonic and Quantum Technologies, University of Otago, Dunedin, New Zealand*
[3]*GPPMM group, XLIM, UMR 7252 Université de Limoges, 123 Avenue Albert Thomas, 87060 Limoges Cedex, France*

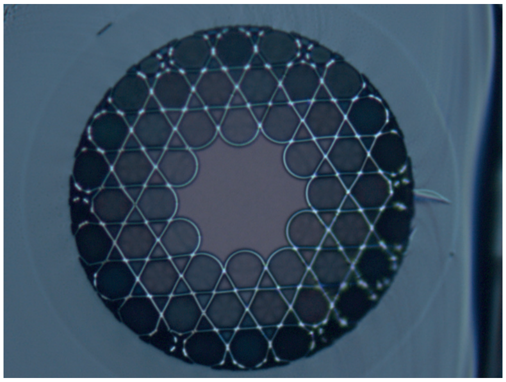

FIG. 1. Hollow-core photonic crystal fiber with a Kagomé cladding lattice and a hypocycloid core-contour [1].

## I. HOLLOW CORE FIBER

Our fiber is an inhibited-coupling [2] guiding hollow-core photonic crystal fiber (HC-PCF) with a Kagomé cladding lattice [3], and a hypocycloid core-contour [4] (shown in Fig. 1). The fiber has an inner diameter of 60 $\mu$m, yielding a mode field diameter of about 42 $\mu$m. Due to its intrinsic optical guidance mechanism akin to a quasi-bound state in the continuum [2], the HC-PCF is multimode in principle. However, because the coupling inhibition between the core and the cladding modes is stronger with the fundamental core-mode [5, 6], the fiber can operate in a single mode fashion. We have confirmed the single mode guiding for the relevant wavelengths by measuring the near and far field profile of the light coupled through the fiber. Furthermore, the choice of our HC-PCF is motivated by its combination of low loss transmission, low birefringence and broadband guidance that covers all the necessary working wavelength of the experiment.

We prepare our HC-PCF before inserting it into the main vacuum chamber by evacuating and cleaning it in a separate vacuum system. To this end, we perform the following cleaning sequence: We flush the vacuum chamber with nitrogen, re-evacuate it down to below $10^{-8}$ mbar and bake out the whole system. This sequence is repeated two times. This preparation should improve the transport of our cold atoms into the fiber, as very few residual particles remain inside the fiber core.

## II. SAMPLE PREPARATION

Rubidium 87 atoms are prepared in a 2D-3D-magneto-optical trap configuration and are loaded into the red-detuned standing wave dipole trap, which is coupled through the atomic cloud into the HC-PCF. The temperature of the atoms of a few tens of $\mu$K is sufficiently lower than the dipole trap depth of $\sim 500$ $\mu$K. When the atoms have been transported in front of the fiber tip, they have heated up to $\sim 300$ $\mu$K. However, the trap depth in front of the fiber tip has also increased to $\sim 1.7$ mK, taking into account that the dipole laser power has been ramped down to 50%, so that the atoms can still be trapped. The lifetime in the optical lattice in front of the fiber tip is about 200 ms. Outside the fiber, number, lifetime and temperature of the atoms are measured using standard absorption imaging.

We also estimate the size of our atomic sample using absorption images by fitting a Gaussian density profile to the atomic cloud. We determine a full Gaussian width in the radial direction of $\sigma_r \sim 40$ $\mu$m at the MOT position and $\sigma_r \sim 30$ $\mu$m in front of the HC-PCF and in the axial direction a full Gaussian width of $\sigma_l \sim 800$ $\mu$m for both positions.

Our MOT is loaded at a distance of 5 mm to the fiber tip. For the measurements shown in the main publication, we typically prepare our atomic sample outside the HC-PCF at a distance of 1 mm to the fiber tip and the sample inside the fiber at a distance of 4 to 5 mm to the fiber tip. In this way, we can compare the in-fiber measurements with an ensemble in similar circumstances. To find the final position after the transport, we determine the center of mass position of the atomic cloud via the applied transport frequency ramp. The final atom position $z$ can be calculated from the maximum applied frequency detuning $\Delta\nu$ between the two lattice beams as follows [7]:

$$z = \left( z_0 + \frac{\lambda\,\Delta\nu\,\Delta t}{4} \right), \tag{1}$$

where $\lambda$ is the lattice wavelength and $\Delta t$ the duration of the frequency ramp. We have confirmed this dependency by determining the atomic center of mass position from absorption images and comparing the values to the ones predicted by eq. 1.

## III. DATA ANALYSIS

The PMT signal is averaged over the duration of each probe pulse. We do not scan the probe frequency during the individual experimental run. Instead, the detuning of the probe beam is changed in each run of the experiment until the whole absorption spectrum is obtained. For each detuning, we average the signal over several runs of the experiment. As in standard absorption imaging, background signals without atoms and without light are taken to normalize the absorption spectra. For all spectra shown in the main publication, 20 consecutive probe pulses have been averaged, unless indicated otherwise. For the time-resolved images, we apply a moving average over 20 neighboring repetitions.

## IV. OPTICAL DEPTH MEASUREMENTS

To understand the optical depth (OD) measurements of $N_{\rm at}$ atoms interacting with the probe beam which is focussing on the fiber tip, we use the following formula [8]:

$$OD = \eta N_{\rm at} \frac{\sigma}{\pi \omega^2}, \qquad (2)$$

where $\omega = \omega_0 \sqrt{1 + \left(\frac{z\lambda}{\pi\omega_0^2}\right)^2}$ is the Gaussian beam waist of the probe beam with minimal beam waist $\omega_0 = 21\ \mu$m inside the HC-PCF, $\sigma$ is the transition strength of the probe transition and $\eta$ is a geometrical factor which describes the overlap between the atomic density distribution and the probe beam. Typical values range from $\eta = 2$ if all atoms are aligned with the beam axis to $\eta = 1$ if the atomic density distribution is also Gaussian with the same beam waist as the probe beam [8]. For simplicity, we assume $\eta$ to stay constant during the transport process. Then, for the same number of atoms, the OD should increase towards the fiber tip as the probe beam waist is reducing towards to its focus.

Fig. 2 shows our OD measurements as function of distance to the fiber tip. As expected, the OD increases as the atoms approach the fiber tip and then stays constant once they have entered the HC-PCF. Our measurements are in good agreement with the theoretical fit corresponding to eq. 2. The first value at the MOT position is the only one to deviate from the fit, which can be explained by the assumption of constant $\eta$ since immediately after loading the overlap between atoms and dipole trap or probe beam can have the largest uncertainty.

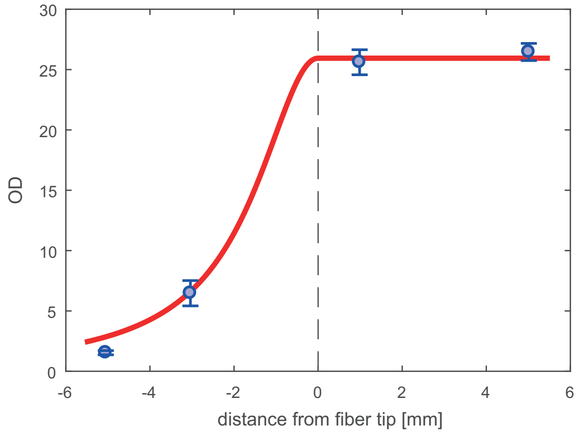


FIG. 2. Experimentally determined optical depth as function of distance from the fiber tip, where the initial MOT position is on the left hand side (averaging over 20 repetitions starting from repetition number 1, statistical error bars), and theoretical fit corresponding to eq. 2.

## V. MEASUREMENT METHODS INSIDE THE FIBER

We determine the temperature of the atoms inside the HC-PCF with a release-and-recapture measurement [8]. For this, the lattice beams are switched off for a variable amount of time $t_{\rm off}$, allowing the hottest atoms to escape the trap region. After the remaining atoms are recaptured in the lattice, the optical depth $OD$ is measured as explained in the previous sections. We then can extract the temperature of the atomic sample by the following fit to the experimental data [8]:

$$OD/OD_0 = 1 - \exp\left(\frac{-\left(R/r_0\right)^2}{1 + \left(v_0/r_0\right)^2 t_{\rm off}^2}\right), \qquad (3)$$

where $R$ is the radius of the fiber core, $OD_0$ the initial optical density, $r_0 = \sigma_r/2$ the radius of the atomic distribution and $v_0$ the most probable speed of the atoms. Using Maxwell-Boltzmann statistics, we can then retrieve the temperature of the atomic ensemble from $v_0 = \sqrt{\frac{2k_B T}{m}}$. Fig. 3 shows a typical measurement with atoms about 5 mm inside the fiber. Here, we measure a temperature of 500 $\mu$K, which is typical for the atoms inside the fiber. In a separate measurement, we have investigated the different heating mechanisms during the transport of the cold atoms and have found heating due to the increased scattering at increasing dipole trap depth close to the fiber tip to be the main factor. We assume this to be the case also inside the HC-PCF. From the fit, we further determine $\sigma_r \sim 16\ \mu$m, which means that the atoms are spread over most of the trapping volume ($\omega_0 = 21\ \mu$m). Note that in this measurement only the on resonance transmission T and thus the on resonance $OD = -ln(T)$ is measured

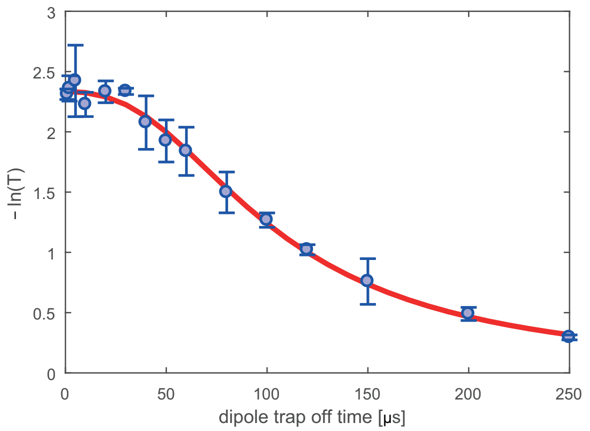


FIG. 3. Release and recapture measurement to determine the temperature inside the hollow core fiber: On resonance optical depth as function of the dipole trap off time (averaging over 10 repetitions starting from repetition number 1, statistical error bars) and theoretical fit corresponding to eq. 3.

instead of taking the full absorption profile, which explains why the values are lower than in the previous measurements. We validate this measurement technique by comparing the temperature values obtained outside the fiber with the normal time-of-flight imaging technique, where we see a good agreement. The lifetime of between 120 ms and 180 ms (determined by OD measurements after a variable hold time in the lattice) is comparable to the measurements at the fiber tip, determined using standard absorption imaging, as given in section II.

* Corresponding author: windpass@uni-mainz.de


[1] Courtesy of the research group of F. Benabid.

[2] F. Couny, F. Benabid, P. J. Roberts, P. S. Light, and M. G. Raymer, Science **318**, 1118 (2007).

[3] F. Benabid, J. C. Knight, G. Antonopoulos, and P. S. J. Russell, Science **298**, 399 (2002).

[4] Y. Y. Wang, N. V. Wheeler, F. Couny, P. J. Roberts, and F. Benabid, Opt. Lett. **36**, 669 (2011).

[5] B. Debord, M. Alharbi, T. Bradley, C. Fourcade-Dutin, Y. Wang, L. Vincetti, F. Gérôme, and F. Benabid, Opt. Express **21**, 28597 (2013).

[6] M. Alharbi, T. Bradley, B. Debord, C. Fourcade-Dutin, D. Ghosh, L. Vincetti, F. Gérôme, and F. Benabid, Opt. Express **21**, 28609 (2013).

[7] D. Schrader, S. Kuhr, W. Alt, M. Müller, V. Gomer, and D. Meschede, Appl. Phys. B **73**, 819 (2001).

[8] M. Bajcsy, S. Hofferberth, T. Peyronel, V. Balic, Q. Liang, A. S. Zibrov, V. Vuletic, and M. D. Lukin, Phys. Rev. A **83**, 063830 (2011).
